# Supplementary material for: Experimental Demonstration Of Scanned Spin-Precession Microscopy
Source: arXiv:1211.7118 source file (2012-11-29)
Supplement: Supplementary file 1 [file SSPM_SI_bbl.tex]

\begin{thebibliography}{2}
\expandafter\ifx\csname natexlab\endcsname\relax\def\natexlab#1{#1}\fi
\expandafter\ifx\csname bibnamefont\endcsname\relax
  \def\bibnamefont#1{#1}\fi
\expandafter\ifx\csname bibfnamefont\endcsname\relax
  \def\bibfnamefont#1{#1}\fi
\expandafter\ifx\csname citenamefont\endcsname\relax
  \def\citenamefont#1{#1}\fi
\expandafter\ifx\csname url\endcsname\relax
  \def\url#1{\texttt{#1}}\fi
\expandafter\ifx\csname urlprefix\endcsname\relax\def\urlprefix{URL }\fi
\providecommand{\bibinfo}[2]{#2}
\providecommand{\eprint}[2][]{\url{#2}}

\bibitem[{\citenamefont{Otsubo et~al.}(1976)\citenamefont{Otsubo, Oda, Kumabe,
  and Miki}}]{Otsubo01011976}
\bibinfo{author}{\bibfnamefont{M.}~\bibnamefont{Otsubo}},
  \bibinfo{author}{\bibfnamefont{T.}~\bibnamefont{Oda}},
  \bibinfo{author}{\bibfnamefont{H.}~\bibnamefont{Kumabe}}, \bibnamefont{and}
  \bibinfo{author}{\bibfnamefont{H.}~\bibnamefont{Miki}},
  \bibinfo{journal}{Journal of The Electrochemical Society}
  \textbf{\bibinfo{volume}{123}}, \bibinfo{pages}{676} (\bibinfo{year}{1976}),
  \eprint{http://jes.ecsdl.org/content/123/5/676.full.pdf+html},
  \urlprefix\url{http://jes.ecsdl.org/content/123/5/676.abstract}.

\bibitem[{\citenamefont{Furis et~al.}(2007)\citenamefont{Furis, Smith, Kos,
  Garlid, Reddy, Palmstrom, Crowell, and Crooker}}]{Furis:2007p479}
\bibinfo{author}{\bibfnamefont{M.}~\bibnamefont{Furis}},
  \bibinfo{author}{\bibfnamefont{D.~L.} \bibnamefont{Smith}},
  \bibinfo{author}{\bibfnamefont{S.}~\bibnamefont{Kos}},
  \bibinfo{author}{\bibfnamefont{E.~S.} \bibnamefont{Garlid}},
  \bibinfo{author}{\bibfnamefont{K.~S.~M.} \bibnamefont{Reddy}},
  \bibinfo{author}{\bibfnamefont{C.~J.} \bibnamefont{Palmstrom}},
  \bibinfo{author}{\bibfnamefont{P.~A.} \bibnamefont{Crowell}},
  \bibnamefont{and} \bibinfo{author}{\bibfnamefont{S.~A.}
  \bibnamefont{Crooker}}, \bibinfo{journal}{New J. Phys.}
  \textbf{\bibinfo{volume}{9}}, \bibinfo{pages}{347} (\bibinfo{year}{2007}),
  \urlprefix\url{http://iopscience.iop.org/1367-2630/9/9/347/}.

\end{thebibliography}
